# Supplementary material for: Mind the Gap? Not for SVP Hardness under ETH!
Source: arXiv:2504.02695 source file (2026-04-21)
Supplement: Supplementary file 1 [file appendix.tex]

\section{Proof of \Cref{claim:SvpGadgetParameter}}
\label{sec:svpGadgetParamProof}

\claimSvpGadgetParam*

\begin{proof}
    For the first inequality,
    \begin{align*}
        r^p-1-r'^p&= \left(1-\frac{\delta}{2} \right)\frac{ 2r'^p}{\delta} - r'^p =2\frac{(1-\delta)}{\delta}r'^p= (\alpha r^\dagger)^p;
    \end{align*}
    Now we will prove the second inequality.  Since $r'^p=\order{m}$, hence WLOG, we can assume $(1+\delta/100)\leq r'^p/10$, which implies,
    \begin{align*}
        (\gamma r)^p &\leq \left(1+\delta/100\right)\left(1+\left(1-\frac{\delta}{2}\right)\frac{2r'^p}{\delta}\right);\\
        &\leq \frac{ r'^p}{10}+\left(1+\delta/100\right)\left(\left(1-\frac{\delta}{2}\right)\frac{2r'^p}{\delta}\right);\\
        & \leq \paren{\frac{\delta}{10}+\paren{1+\frac{\delta}{100}}\paren{2-\delta}}\left(\frac{r'^p}{\delta}\right);\\
        &=\paren{2-\frac{22}{25}\delta-\frac{\delta^2}{100}}\paren{\frac{r'^p}{\delta}};\\
        &< \paren{\frac{2r'^p}{\delta}};\\
        &= (\alpha r^\dagger)^{p}.
    \end{align*}
    For proving the third inequality we will use the fact $\gamma^p \leq 1+\delta\cdot \frac{(\sqrt{\gamma'}-1)^2}{2}$ and $\gamma'\geq 1$. Again, since $r'^p=\order{m}$ , WLOG we can assume that, $\frac{\delta r'^p}{2}\geq \gamma^p$. Hence we get,
    \begin{align*}
        (\gamma r)^p &\leq \paren{\frac{2r'^p}{\delta}}\paren{\paren{1-\frac{\delta}{2}}\paren{1+\delta\cdot \frac{(\sqrt{\gamma'^p}-1)^2}{2}}}+\gamma^p;\\
        &= \paren{\frac{2r'^p}{\delta}} \paren{\paren{1-\delta\sqrt{\gamma'^p}}+\paren{\frac{\delta \gamma'^p}{2}+\frac{\delta^2 \sqrt{\gamma'^p
        }}{4}}-\paren{\frac{\delta(\delta+\delta \gamma'^p)}{4}}}+\gamma^p;\\
        &\leq \paren{\frac{2r'^p}{\delta}} \paren{\paren{1-\delta\sqrt{\gamma'^p}} + \frac{\delta \gamma'^p}{2} -\frac{\delta^2}{4}}+\gamma^p;\\
        &=(1 - \delta\sqrt{\gamma'^p}) (\alpha r^{\dagger})^p+(\gamma'r)^p- \frac{\delta r'^p}{2}+\gamma^p;\\
        &\leq (1 - \delta\sqrt{\gamma'^p}) (\alpha r^{\dagger})^p+(\gamma'r)^p .
    \end{align*}
This concludes the proof of the claim.
\end{proof}
